# Supplementary material for: SF(DA)$^2$: Source-free Domain Adaptation Through the Lens of Data Augmentation
Source: arXiv:2403.10834 source file (2024-03-16)
Supplement: Supplementary file 1 [file Supplementary.tex]

{\footnotesize
\begin{align}
\boldsymbol{\mu}^{(t)}_j &= \frac{n^{(t-1)}_j \boldsymbol{\mu}^{(t-1)}_j + m^{(t)}_j \boldsymbol{\mu}'^{(t)}_j}{n^{(t-1)}_j + m^{(t)}_j} \\
\Sigma^{(t)}_j &= \frac{n^{(t-1)}_j \Sigma^{(t-1)}_j + m^{(t)}_j \Sigma'^{(t)}_j}{n^{(t-1)}_j + m^{(t)}_j} + \frac{m^{(t)}_j + n^{(t-1)}_j m^{(t)}_j (\boldsymbol{\mu}^{(t-1)}_j - \boldsymbol{\mu}'^{(t)}_j) (\boldsymbol{\mu}^{(t-1)}_j - \boldsymbol{\mu}'^{(t)}_j )^T}{(n^{(t-1)}_j + m^{(t)}_j)^2}\\
n^{(t)}_j &= n^{(t-1)}_j + m^{(t)}_j
\end{align}
}

visda는 데이터 수가 많고 클래스 수가 적음
office-home, domainNet은 데이터 수가 적고 클래스 수가 많음
이러한 데이터의 경우 배치 내에 0~1개 데이터만 같은 클래스고, 나머지는 다른 클래스임
contrastive learning에서 같은 클래스 데이터를 밀어내는게 ~효과를 유발해서 성능을 저하시킴
그래서 필터링이 필요함
